# Supplementary material for: Behavior Transformers: Cloning $k$ modes with one stone
Source: arXiv:2206.11251 source file (2022-10-11)
Supplement: Supplementary file 1 [file disk_environments.tex]

\section{Environments}
\label{sec:appendix_environments}
\paragraph{Gym Experiments} We derive all environments used in the experiments in this paper from OpenAI Gym \citep{brockman2016openai} MuJoCo tasks. Namely, we use the HalfCheetah-v3 and Hopper-v3 environments for 2d locomotion tasks and Swimmer-v3 and Ant-v3 environments for the 3d locomotion tasks (see Figure~2 for the agent morphologies).

Since we aim to train primitives, we want policies that perform well regardless of the global states of the agent (global position etc.), only depending on local states (join angles etc.). Thus, we train our agents and each of our baselines with a maximum episode length of $100$ ($200$ for Swimmer only), while we test them with a maximum episode length of $500$ for static or the block environments and $200$ for the broken leg environments.

As our projection function $\sigma$, we measured the $x$ velocity of the agent in 2d environments, and the $(x, y)$ velocity of the agent in 3d environments. We made $\sigma(s)$ available to the intrinsic reward calculation functions of both our methods and the baselines. 

\paragraph{Block Experiments} For our block experiment set, we implemented the blocks as  immovable spheres of radius $3$ at a distance $10$ from origin. We dynamically added $40$ blocks at the environment creation, and deleted them with the MuJoCo interface available in Gym. The blocks were all added before the agent took the first step in the environment, and removed over the agents' lifetime as described in Section~4.3.
The blocks were always removed counter-clockwise, following the trajectory of $(\cos \frac{2 \pi t}{T}, \sin \frac{2 \pi t}{T})$ over $t \in [0, T]$, where $t$ is the current timestep and $T$ is the total timestep for training.

\paragraph{Broken Leg Experiments} For our broken leg experiment set, we implemented a broken leg as a leg where no actions have any effect. We switch which leg is broken every 1M steps, and train all skills for a total of 10M steps in both Off-DADS and \method{}.

\begin{figure}[ht]
    \centering
    \includegraphics[width=\linewidth]{iclr2022/figs/disk_broken_legs_appendix.pdf}
    \caption{Skills learned by \method{}, evaluated with each of the legs broken. The legs are numbered such that the final leg is numbered \#4}
    \label{fig:disk_all_broken}
\end{figure}
\begin{figure}[ht]
    \centering
    \includegraphics[width=\linewidth]{iclr2022/figs/dads_broken_legs_appendix.png}
    \caption{Skills learned by Off-DADS at the end of 10M steps, evaluated with each of the legs broken. The legs are numbered such that the final leg is numbered \#4,}
    \label{fig:dads_all_broken}
\end{figure}
% \begin{figure}[ht]
%     \centering
%     \includegraphics[width=\linewidth]{iclr2022/figs/18100.png}
%     \caption{Skills learned by Off-DADS at the end of 9M steps, evaluated with each of the legs broken. Compared to this agent, the agent in Fig. ~\ref{fig:dads_all_broken} performs worse, which is an instance of catastrophic forgetting.}
%     \label{fig:dads_all_broken_9m}
% \end{figure}

\paragraph{Hierarchical Experiments} For the hierarchical environments, we use the Ant-v3 environment in a goal-conditioned manner. The goals are sampled from $[-15, 15]^2$ uniformly, and the hierarchical agent can take $100$ steps to reach as close to the goal as possible. At each step of the hierarchical agent, it chooses a skill, which is then executed for 10 timesteps in the underlying environment. So, in total, the agent has $1000$ timesteps to reach the goal. At every timestep, the agent is given a dense reward of $-\|x - g\|_2$, where $x$ is the current location of the agent, and $g$ is the location of the goal. On each step, the hierarchical agent gets the sum of the goal conditioned reward from the 10 timesteps in the underlying environment.

All the hierarchical agents were trained with the \texttt{stable-baselines3} package \citep{stable-baselines3}. We used their default PPO agent for all the downstream set of skills, and trained the hierarchical agent for a total $500\,000$ environment steps.
