# Supplementary material for: Behavior Transformers: Cloning $k$ modes with one stone
Source: arXiv:2206.11251 source file (2022-10-11)
Supplement: Supplementary file 2 [file disk_math.tex]

\section{Further Mathematical Details}
\label{sec:appendix_math}
\subsection{Expansion and Derivation of Objectives}
The objective function $\gF (\theta)$, as defined in Equation~1, is the source from where we derive our incremental objective function, reproduced here.

\begin{equation*}
    \gF(\theta) = I(S;Z) + \mathcal{H}(A|S,Z)
\end{equation*}

We can expand the first term in Equation~1 as

\begin{align*}
    I(S;Z) &\equiv H(S) - H(S\mid Z)
\end{align*}
by definition of mutual information. Now, once we assume $Z$ is a discrete variable, the second part of this equation becomes 
\begin{align*}
    \mathcal H(S\mid Z) &\equiv \sum_{z_m} p(z_m) \mathcal H(S \mid Z = z_m) \\
    &= \expect_{z_m \sim p(z_m)} \left [ \mathcal H(S \mid Z = z_m) \right ]
\end{align*}
And thus we have 
\begin{align*}
    I(S; Z) &= \mathcal{H}(S) - \expect_{z_m \sim p(z_m)} \left [ \mathcal H(S \mid Z = z_m) \right ] \\
    &= \expect_{z_m \sim p(z_m)} \left [ \mathcal{H}(S) - \mathcal H(S \mid Z = z_m) \right ] \\
\end{align*}

But the term inside the expectation is the definition of information gain (not to be confused with KL divergence), defined by
\begin{align*}
    IG(S; Z = z_m) &\equiv \mathcal{H}(S) - \mathcal H(S \mid Z = z_m)
\end{align*}
Thus, we arrive at
\begin{align*}
    I(S; Z)
    &= \expect_{z_m \sim p(z_m)} \left [ IG(S; Z = z_m) \right ] \\
\end{align*}

Similarly, by definition of conditional entropy, we can expand the second part of the Equation~1
\begin{align*}
    \mathcal H(A\mid S, Z) &\equiv \sum_{z_m} p(z_m) \mathcal H(A \mid S, Z = z_m) \\
    &= \expect_{z_m \sim p(z_m)} \left [ \mathcal H(A \mid S, Z = z_m) \right ]
\end{align*}

Thus, we can convert Equation~1 into
\begin{align*}
    \gF(\theta) &= I(S;Z) + \mathcal{H}(A|S,Z) \\
    &= \expect_{z_m \sim p(z_m)} \left [ IG(S; Z = z_m) \right ] + \expect_{z_m \sim p(z_m)} \left [ \mathcal H(A \mid S, Z = z_m) \right ] \\
    &= \expect_{z_m \sim p(z_m)} \left [ IG(S; Z = z_m)   + \mathcal H(A \mid S, Z = z_m) \right ]
\end{align*}

If we assume a uniform prior over our skills, which is another assumption made by \cite{diversity}, and also assume we are trying to learn $M$ skills in total, we can further expand Equation~1 into:
\begin{align*}
    \gF(\theta)
    &= \frac{1}{M}  \sum _{m = 1}^M \left [ IG(S; Z = z_m)   + \mathcal H(A \mid S, Z = z_m) \right ]
\end{align*}
Ignoring the number of skills term (which is constant over a single skills' learning period) gives us exactly Equation~3, which was:
\begin{align*}
    \gF(\theta)
    &:= \sum _{m = 1}^M \left [ IG(S; Z = z_m)   + \mathcal H(A \mid S, Z = z_m) \right ]
\end{align*}

Now, under our framework, we assume that skills $1, 2, \cdots, M-1$ has been learned and fixed, and we are formulating an objective for the $M$th skill. As a result, we can ignore the associated Information Gain and action distribution entropy terms from skills $1, 2, \cdots, M-1$, and simplify our objective to be:
\begin{align*}
    \gF(\theta)
    &:= IG(S; Z = z_M)   + \mathcal H(A \mid S, Z = z_M)  \\
    &= \mathcal H(S) - \mathcal H(S \mid Z = z_M) + \mathcal H(A \mid S, Z = z_M)
\end{align*}
which is exactly the same objective we defined in Equation~5.

\subsection{Point-based Nearest Neighbor Entropy Estimation}
In our work, we use an alternate approach, first shown by ~\citet{singh2003nearest}, to estimate the entropy of a set of points. This method gives us a non-parametric Nearest Neighbor (NN) based entropy estimator:
\begin{align*}
    \hat{\mathbb{H}}_{k,\mX}(p) &= -\frac{1}{N}\sum_{i=1}^N\ln\frac{k\Gamma(q/2+1)}{N \pi^{q/2} R_{i,k,\mX}^q } + C_k,
\end{align*}
where $\Gamma$ is the gamma function, $C_k=\ln k -\frac{\Gamma'(k)}{\Gamma(k)}$ is the bias correction term, and  $R_{i,k,\mX}=\|\vx_i - \mathrm{NN}_{k,\mX}(\vx_i)\|$ is the Euclidean distance between $\vx_i$ and its $k^{\text{th}}$ nearest neighbor from the dataset $\mX$, defined as $\mathrm{NN}_{k,\mX}(\vx_i)$.

The term inside the sum can be simplified as 
\begin{align*}
    \ln\frac{k\Gamma(q/2+1)}{N \pi^{q/2} R_{i,k,\mX}^q } &= \ln\frac{k\Gamma(q/2+1)}{N \pi^{q/2} } - \ln R_{i,k,\mX}^q \\&= \ln\frac{k\Gamma(q/2+1)}{N \pi^{q/2} } - q\ln R_{i,k,\mX}\\
    &= \ln\frac{k\Gamma(q/2+1)}{N \pi^{q/2} } - q\ln \|
    \vx_i - \mathrm{NN}_{k,\mX}(\vx_i)\|.
\end{align*}

Here, $\ln\dfrac{k\Gamma(q/2+1)}{N \pi^{q/2} }$ is a constant term independent of $\vx_i$. If we ignore the this term and the bias-correction term $C_k$ and the constant, we get 
\begin{align*}
\label{eqn:entropy}
    \hat{\mathbb{H}}_{k,\mX}(p) &\propto \sum_{i=1}^N \ln \|
    \vx_i - \mathrm{NN}_{k,\mX}(\vx_i)\|.
\end{align*}
Which is the formulation we use in this work. This estimator is shown to be asymptotically unbiased and consistent in~\citet{singh2003nearest}.

\subsection{Hausdorff Distance}\label{app:hausdorff}

In our work, to compare between two algorithms learning skills on the same environment, we used a metric based on Hausdorff distance. 
Hausdorff distance, also known as the Hausdorff metric or the Pompeiu–Hausdorff distance, is a metric that measures the distance between two subsets of a metric space. 
Informally, we think of two sets in a metric space as close in the Hausdorff distance if every point of either set is close to some point of the other set. 
The Hausdorff distance is the longest distance one can force you to travel by choosing a point adversarially in one of the two sets, from which you have to travel to the other set. Put simply, it is the greatest of all the distances from a point in one set to the nearest point in the other.

Mathematically, given two subsets $A$ and $B$ of a metric space $(M, d)$ we define Hausdorff distance $d_H{(A, B)}$ as:
\[d_H(A, B) = \max\left \{ \sup_{a\in A} d(a, B), \sup_{b\in B} d(b, A)\right \}\]
Where $\sup$ represents the supremum, $d(x, Y) = \inf_{y\in Y}d(x, y)$ is the distance between a point and another set, and $\inf$ represents the infimum.

Given a set of skills, we calculate the diversity of one skill over all other skills by calculating the Hausdorff distance between that skill's trajectory end $(x, y)$ location, and the terminal $(x, y)$ locations of all other trajectories. Intuitively, a skill has high Hausdorff distance if the end states it generates is far away from other skills' endpoints. Similarly, a high average Hausdorff distance for skills from an algorithm means that the algorithm's generated skills on average have a high distance from each other, which is a desirable property for an algorithm which needs to generate diverse skills.
