# Supplementary material for: Behavior Transformers: Cloning $k$ modes with one stone
Source: arXiv:2206.11251 source file (2022-10-11)
Supplement: Supplementary file 3 [file reinforcement_learning.tex]

\section{Reinforcement learning}
\label{sec:appendix_rl}

% \section{Reinforcement learning}
% \label{sec:appendix_rl}
% \lpnote{we can skip this section and refer reader to appendix.} 
In our continuous-control RL setting, an agent receives a state observation $s_t \in \mathcal{S}$ from the environment and applies an action $a_t \in \mathcal{A}$ according to policy $\pi$. In our setting, where the policy is stochastic, the policy returns a distribution $\pi(s_t)$, and we sample a concrete action $a_t \sim \pi(s_t)$. The environment returns a reward for every action $r_t$. The goal of the agent is to maximize expected cumulative discounted reward $\E_{s_{0:T},a_{0:T-1},r_{0:T-1}}\left[\sum_{t=0}^{T-1} \gamma^t r_t\right]$ for discount factor $\gamma$ and horizon length $T$.

On-policy RL ~\citep{schulman2015trust,kakade2002natural,williams1992simple} optimizes $\pi$ by iterating between data collection and policy updates. It hence requires new on-policy data every iteration, which is expensive to obtain. On the other hand, off-policy reinforcement learning retains past experiences in a replay buffer and is able to re-use past samples. Thus, in practice, off-policy algorithms have been found to achieve better sample efficiency \citep{lillicrap2015continuous,haarnoja2018soft}. For our experiments we use SAC~\citep{haarnoja2018soft} as our base RL optimizer due to its implicit maximization of action distribution entropy, sample efficiency, and fair comparisons with baselines that also build on top of SAC. However, we note that our framework is compatible with any standard off-policy RL algorithm that maximizes the entropy of the action distribution $\pi(\cdot)$ either implicitly or explicitly.

\paragraph{Soft Actor-Critic} 
The Soft Actor-Critic (SAC)~\citep{haarnoja2018soft} is an off-policy model-free RL algorithm that instantiates an actor-critic framework by learning a state-action value function $Q_\theta$, a stochastic policy $\pi_\theta$  and a temperature $\alpha$ over a discounted infinite-horizon MDP $(\gX, \gA, P, R, \gamma, d_0)$ by optimizing a $\gamma$-discounted maximum-entropy objective~\citep{ziebart2008maximum}. With a slight abuse of notation, we define both the actor and critic learnable parameters by $\theta$. SAC parametrizes  the actor policy $\pi_\theta(\va_t|\vx_t)$ via a $\mathrm{tanh}$-Gaussian defined  as $
\va_t = \mathrm{tanh}(\mu_\theta(\vx_t)+ \sigma_\theta(\vx_t) \epsilon)$, where $\epsilon \sim \gN(0, 1)$, $\mu_\theta$ and $\sigma_\theta$ are parametric mean and standard deviation. The SAC's critic $Q_\theta(\vx_t, \va_t$) is parametrized as an MLP neural network.

The policy evaluation step  learns  the critic $Q_\theta(\vx_t, \va_t)$ network by optimizing the one-step soft Bellman residual:
\begin{align*}
    \gL_Q(\gD) &= \E_{\substack{( \vx_t,\va_t, \vx_{t+1}) \sim \gD \\ \va_{t+1} \sim \pi(\cdot|\vx_{t+1})}}[(Q_\theta(\vx_t, \va_t) - y_t)^2]\text{ and}\\
    y_t &= R(\vx_t, \va_t) + \gamma [Q_{\theta'}(\vx_{t+1}, \va_{t+1}) - \alpha \log \pi_\theta(\va_{t+1}|\vx_{t+1})] ,
\end{align*}
where $\gD$ is a replay buffer of transitions, $\theta'$ is an exponential moving average of $\theta$ as done in~\citep{lillicrap2015continuous}. SAC uses clipped double-Q learning~\citep{van2016deep, fujimoto2018addressing}, which we omit from our notation for simplicity but employ in practice.

The policy improvement step then fits the actor $\pi_\theta(\va_t|\vs_t)$ network by optimizing the following objective:
\begin{align*}
    \gL_\pi(\gD) &= \E_{\vx_t \sim \gD}[ \KL(\pi_\theta(\cdot|\vx_t) || \exp\{\frac{1}{\alpha}Q_\theta(\vx_t, \cdot)\})].
\end{align*}
Finally, the temperature $\alpha$ is learned with the loss:
\begin{align*}
    \gL_\alpha(\gD) &= \E_{\substack{\vx_t \sim \gD \\ \va_t \sim \pi_\theta(\cdot|\vx_t)}}[-\alpha \log \pi_\theta(\va_t|\vx_t) - \alpha \bar\gH],
\end{align*}
where $\bar\gH \in \R$ is the target entropy hyper-parameter that the policy tries to match, which in practice is set to  $\bar\gH=-|\gA|$.
The overall optimization objective of SAC equals to:
\begin{align*}
    \mathcal{L}_\mathrm{SAC}(\gD) &= \gL_\pi(\gD) + \gL_Q(\gD) + \gL_\alpha(\gD).
\end{align*}
